# Supplementary material for: Lingjing: A Simulation Testbed for Multi-Agent Embodied Tasks in Open-Ended Cities
Source: arXiv:2608.08045 source file (2026-08-08)
Supplement: Supplementary file 2 [file F_reproducibility.tex]

\section{Reproducibility Checklist}
\label{app:repro}

\subsection{Software stack}

\begin{itemize}[leftmargin=*,itemsep=2pt]
\item Backend: Python 3.11, FastAPI 0.110, Uvicorn 0.29, websockets 12.x, SQLAlchemy 2.x (sync, two engines), pydantic 2.x.
% 中文翻译：
% 后端：Python 3.11、FastAPI 0.110、Uvicorn 0.29、websockets 12.x、
% SQLAlchemy 2.x（同步、两个 engine）、pydantic 2.x。
\item Agents: LangGraph 0.0.x for the one-shot planners; System/Group/Individual prompt templates call OpenAI-compatible chat completions or a local \texttt{vllm} server when an open-source backbone is used.
% 中文翻译：
% 智能体：one-shot 规划器使用 LangGraph 0.0.x；
% 当使用开源骨干时，System/Group/Individual prompt 模板调用
% OpenAI 兼容 chat completions 或本地 \texttt{vllm} 服务器。
\item Engine: Unreal Engine 5.x on Windows builds; the WebSocket schema (App.~\ref{app:platform:ws}) is the only ABI between the Python backend and the renderer.
% 中文翻译：
% 引擎：Windows 构建上的 Unreal Engine 5.x；
% WebSocket schema（附录~\ref{app:platform:ws}）
% 是 Python 后端与渲染器之间唯一的 ABI。
\item Stream DB: a single SQLite \texttt{data/stream.db} per machine, WAL mode, with periodic \texttt{VACUUM INTO} snapshots produced by the recorder.
% 中文翻译：
% 流数据库：每台机器一个 SQLite \texttt{data/stream.db}，
% 使用 WAL 模式，并由记录器定期生成 \texttt{VACUUM INTO} 快照。
\end{itemize}

\subsection{Hardware setup}

The recommended setup uses three machines: a CPU node hosting the FastAPI backend, a Windows workstation running the Unreal renderer, and an optional GPU node hosting \texttt{vllm} for open-source backbones. Commercial backbones are accessed through OpenAI-compatible HTTP APIs. The engine bridge and SQLite writer are lightweight relative to model inference, but all runs should record host, GPU, provider, and model version metadata with the result file.
% 中文翻译：
% 推荐配置使用三台机器：一台承载 FastAPI 后端的 CPU 节点、
% 一台运行 Unreal 渲染器的 Windows 工作站，
% 以及一台可选 GPU 节点用于通过 \texttt{vllm} 托管开源骨干。
% 商业骨干通过 OpenAI 兼容 HTTP API 访问。
% 相比模型推理，引擎桥接和 SQLite 写入器较轻量，
% 但所有运行都应在结果文件中记录主机、GPU、provider 和模型版本元数据。

\subsection{Seeds and determinism}

We use three master seeds $\{007,019,041\}$. Each seed pins (i) the backbone's \texttt{seed} parameter where supported, (ii) the scenario sampler's NumPy seed (scene id, traffic schedule), and (iii) the engine's pseudo-random subsystems (pedestrian routing, weather fluctuation). Engine animation is not bit-deterministic across re-runs of the same seed; however, the \texttt{getObservation} payloads we log are reproducible to within sensor-noise tolerances, and the trajectory recorder makes the agent-side execution path exactly reproducible from \texttt{sim\_data.task\_id}.
% 中文翻译：
% 我们使用三个主 seed：$\{007,019,041\}$。
% 每个 seed 固定：（i）骨干在支持时的 \texttt{seed} 参数；
% （ii）场景采样器的 NumPy seed（场景 id、交通日程）；
% （iii）引擎的伪随机子系统（行人路由、天气波动）。
% 在同一 seed 的重复运行之间，引擎动画并非 bit 级确定；
% 但我们记录的 \texttt{getObservation} payload 在传感器噪声容差内可复现，
% 且轨迹记录器使智能体侧执行路径可从 \texttt{sim\_data.task\_id}
% 精确复现。

\subsection{Single-task reproduction recipe}

To reproduce a single benchmark task, for example \(T7\) with GPT-4o on seed
$007$:
% 中文翻译：
% 若要复现单个基准任务，例如在 seed $007$ 上使用 GPT-4o 复现 \(T7\)：

\begin{enumerate}[leftmargin=*,itemsep=2pt]
\item Start the backend: \texttt{uvicorn app.main:app --port 8000} with \texttt{LINGJING\_DB\_PATH=data/lingjing.db}, \texttt{LINGJING\_STREAM\_DB\_PATH=data/stream.db}.
% 中文翻译：
% 启动后端：使用 \texttt{LINGJING\_DB\_PATH=data/lingjing.db}、
% \texttt{LINGJING\_STREAM\_DB\_PATH=data/stream.db}
% 运行 \texttt{uvicorn app.main:app --port 8000}。
\item Start the Unreal renderer, connect as \texttt{ws://.../ws/LJ-ENGINE/eng-01}.
% 中文翻译：
% 启动 Unreal 渲染器，并以 \texttt{ws://.../ws/LJ-ENGINE/eng-01} 连接。
\item Submit the scenario with the task JSON or the corresponding \texttt{run\_case*.py} wrapper.
% 中文翻译：
% 使用任务 JSON 或对应的 \texttt{run\_case*.py} wrapper 提交场景。
\item Submit the planner or runner with \texttt{\{"backbone":"gpt-4o","seed":7\}}; the exact command is recorded beside the result summary.
% 中文翻译：
% 使用 \texttt{\{"backbone":"gpt-4o","seed":7\}} 提交规划器或 runner；
% 精确命令会记录在结果摘要旁边。
\item Re-evaluate or re-stream: \texttt{GET /sim/data/getBySceneId?sceneId=T7} returns the complete \texttt{sim\_data} stream; the evaluator can be re-scored against a different metric via \texttt{POST /api/envs/episodes/T7/rescore}.
% 中文翻译：
% 重新评估或重新流式读取：
% \texttt{GET /sim/data/getBySceneId?sceneId=T7}
% 返回完整 \texttt{sim\_data} 流；
% 评估器可以通过 \texttt{POST /api/envs/episodes/T7/rescore}
% 按不同指标重新评分。
\end{enumerate}

\paragraph{Public release.}
We release Lingjing under a permissive open-source licence, including the scenario JSON of every task in Table~\ref{tab:tasks}, the LangGraph planner code, the prompt templates of App.~\ref{app:vla:prompts}, the evaluator stack (\path{app/modules/envs/evaluators/}), and the trajectory recorder. The Unreal Engine assets that produce the visual stream are distributed separately, but the entire benchmark, including all attribution metrics, is computable from the \texttt{sim\_data} stream alone; replaying a recorded episode end-to-end therefore requires only the open-source Python stack and the released \texttt{stream.db} files we ship with the bench.
% 中文翻译：
% 公开发布。我们以宽松开源许可证发布 Lingjing，
% 包括表~\ref{tab:tasks} 中每个任务的场景 JSON、LangGraph 规划器代码、
% 附录~\ref{app:vla:prompts} 的 prompt 模板、评估器栈
% （\path{app/modules/envs/evaluators/}）和轨迹记录器。
% 产生视觉流的 Unreal Engine 资产会单独分发，
% 但整个基准（包括所有归因指标）都可以仅从 \texttt{sim\_data} 流计算；
% 因此，端到端回放一个已记录 episode 只需要开源 Python 栈
% 和我们随基准发布的 \texttt{stream.db} 文件。
